# Supplementary material for: SD-DiT: Unleashing the Power of Self-supervised Discrimination in Diffusion Transformer
Source: arXiv:2403.17004 source file (2024-03-25)
Supplement: Supplementary file 1 [file supp.tex]

\documentclass[10pt,twocolumn,letterpaper]{article}
\input{preamble}

\usepackage[review]{cvpr}

\usepackage[utf8]{inputenc} % allow utf-8 input
\usepackage[T1]{fontenc}    % use 8-bit T1 fonts
\usepackage{hyperref}       % hyperlinks
\usepackage{url}            % simple URL typesetting
\usepackage{booktabs}       % professional-quality tables
\usepackage{amsfonts}       % blackboard math symbols
\usepackage{nicefrac}       % compact symbols for 1/2, etc.
\usepackage{microtype}      % microtypography
\usepackage{xcolor}         % colors
\input{def.set}

%math
\usepackage{amsthm}
\usepackage{mathtools}
\usepackage{algorithm}
\usepackage{bbding}
\usepackage{listings}
\usepackage{subcaption}

\usepackage{pifont}
\usepackage{color}
\usepackage{amssymb}
\usepackage{graphicx}
\usepackage{wrapfig}
\usepackage{makecell}
\usepackage{colortbl}
\usepackage{multirow}
\usepackage{fixltx2e}
\usepackage{subcaption}
\usepackage{amsmath}
\usepackage{etoolbox}
\usepackage{multicol}
\usepackage{refcount}
\usepackage{enumitem}
\usepackage{hyperref}

\usepackage{colortbl}\definecolor{mygray}{gray}{.9}

\usepackage[capitalize]{cleveref}
\crefname{section}{Sec.}{Secs.}
\Crefname{section}{Section}{Sections}
\Crefname{table}{Table}{Tables}
\crefname{table}{Tab.}{Tabs.}

\usepackage{color}

\usepackage{listings}
\usepackage{newfloat}
%New colors defined below
\definecolor{codegreen}{rgb}{0.5,0.6,0.6}
\definecolor{codegray}{rgb}{0.5,0.5,0.5}
\definecolor{codepurple}{rgb}{0.58,0,0.82}
\definecolor{backcolour}{rgb}{0.95,0.95,0.92}

\usepackage{algorithm}
\usepackage{algorithmic}
\lstdefinestyle{mystyle}{
  %backgroundcolor=\color{backcolour}, 
  commentstyle=\color{codegreen},
  keywordstyle=\color{magenta},
  numberstyle=\tiny\color{codegray},
  stringstyle=\color{codepurple},
  basicstyle=\linespread{0.8}\ttfamily\scriptsize,
  breakatwhitespace=false,         
  breaklines=true,                 
  captionpos=b,                    
  keepspaces=false,  
  %numbers=left,                    
  %numbersep=5pt,                  
  showspaces=false,                
  showstringspaces=false,
  showtabs=false,                  
  tabsize=1
}
%"mystyle" code listing set
\lstset{style=mystyle}
\newsavebox{\mycode}

\usepackage{etoolbox}
\makeatletter
\AfterEndEnvironment{algorithm}{\let\@algcomment\relax}
\AtEndEnvironment{algorithm}{\kern2pt\hrule\relax\vskip3pt\@algcomment}
\let\@algcomment\relax
\newcommand\algcomment[1]{\def\@algcomment{\footnotesize#1}}
\renewcommand\fs@ruled{\def\@fs@cfont{\bfseries}\let\@fs@capt\floatc@ruled
  \def\@fs@pre{\hrule height.8pt depth0pt \kern2pt}%
  \def\@fs@post{}%
  \def\@fs@mid{\kern2pt\hrule\kern2pt}%
  \let\@fs@iftopcapt\iftrue}
\makeatother
%----------------------------------------------------------

 % *** Enter the Paper ID here

 % *** Enter the CVPR Paper ID here

\begin{document}

\title{SD-DiT: Unleashing the Power of Self-supervised Discrimination \\ in Diffusion Transformer\\---CVPR 2024 Supplementary Material}

	\author{First Author\\
		Institution1\\
		Institution1 address\\
		{\tt\small firstauthor@i1.org}
		% For a paper whose authors are all at the same institution,
		% omit the following lines up until the closing ``}''.
		% Additional authors and addresses can be added with ``\and'',
		% just like the second author.
		% To save space, use either the email address or home page, not both
		\and
		Second Author\\
		Institution2\\
		First line of institution2 address\\
		{\tt\small secondauthor@i2.org}
	}
	\maketitle
    \input src_supp/details
    \input src_supp/algorithm2

\clearpage

    {    
    \small
    \bibliographystyle{ieeenat_fullname}
    \bibliography{main}
    }

%%%%%%%%%%%%%%%%%%%%%%%%%%%%%%%%%%%%%%%%%%%%%%%%%%%%%%%%%%%%

\end{document}
